# Supplementary material for: Best Practices for Data-Efficient Modeling in NLG:How to Train Production-Ready Neural Models with Less Data
Source: arXiv:2011.03877 source file (2020-11-08)
Supplement: Supplementary file 1 [file Appendix.tex]

%
% File Appendix.tex
%
% Contact: feiliu@cs.ucf.edu & liang.huang.sh@gmail.com
%% Based on the style files for COLING-2018, which were, in turn,
%% Based on the style files for COLING-2016, which were, in turn,
%% Based on the style files for COLING-2014, which were, in turn,
%% Based on the style files for ACL-2014, which were, in turn,
%% Based on the style files for ACL-2013, which were, in turn,
%% Based on the style files for ACL-2012, which were, in turn,
%% based on the style files for ACL-2011, which were, in turn, 
%% based on the style files for ACL-2010, which were, in turn, 
%% based on the style files for ACL-IJCNLP-2009, which were, in turn,
%% based on the style files for EACL-2009 and IJCNLP-2008...

%% Based on the style files for EACL 2006 by 
%%e.agirre@ehu.es or Sergi.Balari@uab.es
%% and that of ACL 08 by Joakim Nivre and Noah Smith

\documentclass[11pt]{article}

\usepackage{url}
\usepackage[colorlinks,citecolor=blue,urlcolor=blue,bookmarks=false,hypertexnames=true]{hyperref} 
\usepackage{coling2020}
\usepackage{times}
\usepackage{url}
\usepackage{latexsym}
\usepackage{textcomp}
\usepackage{booktabs} % For formal tables
\usepackage[flushleft]{threeparttable}
\usepackage{multirow}
% \captionsetup[sub]{font=normalsize,labelfont={bf,sf}}
\usepackage{graphicx}
\usepackage{enumitem}
\usepackage{array}
\usepackage{amssymb}
\usepackage{xspace}
\usepackage{mathtools}
\usepackage{xcolor}
\usepackage{pgfplots}
\pgfplotsset{compat=newest}
\usepackage{tabularx}
\usepackage{filecontents}
\usepackage{tikz}
\usepackage{subcaption}
\usepackage{color}
\usepackage{todonotes}
\usepackage{graphicx}
\usepackage{caption}

\begin{document}

\section{Appendix}
\subsection{Detailed Experimental Results}

\begin{table*}[th!]
  \small
  \begin{center}
    \begin{tabularx}{0.99\linewidth}{c|c|ccccc}
    \cline{1-7}
     \multirow{2}{*}{\textbf{Data}}& \multirow{2}{*}{\textbf{Approach}} & \textbf{BLEU} & \textbf{\textsc{Tree}} & \multirow{2}{*}{\textbf{Acceptability}} & \textbf{\textsc{Data}}& \textbf{\textsc{TreeAcc}}\\ 
     &  & \textbf{\textsc{Score}} & \textbf{\textsc{Accuracy}} &  & \textbf{\textsc{Reduction}}& \textbf{\textsc{STDev}}\\
    \cline{1-7}
    \textbf{BASE}   & \textbf{\textsc{S2S}} & 93.3 & 99.8 & - & 0.0 & 0.1 \\
     \cline{1-7}
     \textbf{1PerCB} & \textbf{\textsc{S2S}} & 51.5 & 0.6 & 5.2 & 99.6 & 3.5 \\
     \cline{1-7}
    \textbf{1PerMB} & \textbf{\textsc{S2S}}& 87.0 & 56.2 & 38.1 & 98.3 & 23.9 \\
     \cline{1-7}
    \textbf{5PerMB+Reminder} &  \textbf{\textsc{S2S+JT}}& 92.7 & 99.6 & 93.8 & 93.7 & 1.3 \\
     \cline{1-7}
     \textbf{3PerFB+Reminder} & \textbf{\textsc{S2S+JT}}& 92.7 & 98.1 & 91.7 & 94.0 & 2.0 \\
     \cline{1-7}
     \textbf{1PerFBQ+Reminder} & \textbf{\textsc{S2S+JT}}& 92.6 & 97.6 & 83.5 & 96.1 & 2.8 \\
     \cline{1-7}
     \textbf{1PerFBQ} &  \textbf{\textsc{S2S}}& 91.6 & 85.0 & 67.0 & 96.1 & 16.2 \\
     \cline{1-7}
     \textbf{1PerFB} &  \textbf{\textsc{S2S}}& 92.3 & 91.8 & 75.0 & 97.4 & 28.6 \\
     \cline{1-7}
    \textbf{1PerFBQ} &  \textbf{\textsc{S2S+DDA}}& 92.7 & 93.4 & 77.3 & 96.1 & 14.3 \\
     \cline{1-7}
    \textbf{1PerFB}  & \textbf{\textsc{S2S+DDA}}& 91.6 & 83.8 & 67.0 & 97.4 & 20.9 \\
     \cline{1-7} 
     \textbf{1PerFBQ} &  \textbf{\textsc{BART+DDA}} & 92.5 & 99.8 & 93.8 & 96.1 & 1.3 \\
     \cline{1-7}
      \textbf{1PerFB} &  \textbf{\textsc{BART+DDA}} & 92.8 & 98.4 & 90.7 & 97.4 & 10.0 \\
    \cline{1-7}
    \textbf{1PerFBQ} &  \textbf{\textsc{S2S+KD}} & 92.9 & 99.9 & 94.8 & 96.1 & 0.1 \\
    \cline{1-7}
    \textbf{1PerFB} &  \textbf{\textsc{S2S+KD}} & 93.2 & 99.8 & 92.8 & 97.4 & 0.1 \\
    \cline{1-7}
    \textbf{1PerFBQ}  & \textbf{\textsc{S2S+KD+DDA}}& 92.9 & 99.9 & 94.8 & 96.1 & 0.05 \\
    \cline{1-7}
    \textbf{1PerFB}  & \textbf{\textsc{S2S+KD+DDA}}& 93.2 & 99.8 & 93.8 & 97.4 & 0.1 \\
    \cline{1-7}
    \end{tabularx}
  \end{center}
  \vspace{-0.2cm}
   \caption{Results on all Alarm domain experiments. All metrics are percentages. }
     \label{tab:alarmresultsall}%
     \vspace{-0.5cm}
\end{table*}%

 \vspace{1.5cm}
 
\begin{table*}[bh!]
  \small
  \centering
 %   \begin{tabularx}{0.99\linewidth}{c|c|ccccc}
    \begin{tabularx}{0.85\linewidth}{ @{} c | c | c c c c c @{} }
    \cline{1-7}
     \multirow{2}{*}{\textbf{Data}}& \multirow{2}{*}{\textbf{Approach}} & \textbf{BLEU} & \textbf{\textsc{Tree}} & \multirow{2}{*}{\textbf{Acceptability}} & \textbf{\textsc{Data}}& \textbf{\textsc{TreeAcc}}\\ 
     &  & \textbf{\textsc{Score}} & \textbf{\textsc{Accuracy}} &  & \textbf{\textsc{Reduction}}& \textbf{\textsc{STDev}}\\
    \cline{1-7}
    \textbf{ALL}   & \textbf{\textsc{S2S BASE}} & 95.9 & 100 & - & 0.0 & 0.1 \\
     \cline{1-7}
     \textbf{1PerCB}   & \textbf{\textsc{S2S}} & 76.1 & 12.1 & 1.3 & 99.7 & 4.9 \\
     \cline{1-7}
     \textbf{1PerMB}  &\textbf{\textsc{S2S}} & 92.3 & 80.1 & 61.3 & 94.8 & 16.5 \\
     \cline{1-7}
     \textbf{1PerFBQ} & \textbf{\textsc{S2S}} & 95.4 & 97.7 & 90.0 & 85.0 & 2.5 \\
     \cline{1-7}
     \textbf{1PerFB}  & \textbf{\textsc{S2S}} & 93.5 & 89.1 & 76.7 & 94.0 & 7.6 \\
     \cline{1-7}
    \textbf{1PerFBQ}   & \textbf{\textsc{S2S+DDA}} & 95.7 & 99.6 & 96.7 & 85.0 & 4.8 \\
     \cline{1-7}
    \textbf{1PerFB}   & \textbf{\textsc{S2S+DDA}} & 94.9 & 97.8 & 87.3 & 94.0 & 10.2 \\
     \cline{1-7} 
     \textbf{1PerFBQ}  & \textbf{\textsc{BART+DDA}} & 95.5 & 99.6 & 98.0 & 85.0 & 0.2 \\
     \cline{1-7}
      \textbf{1PerFB}  & \textbf{\textsc{BART+DDA}} & 93.8 & 96.1 & 90.7 & 94.0 & 1.7 \\
    \cline{1-7}
    \textbf{1PerFBQ} & \textbf{\textsc{S2S+KD}} & 95.8 & 99.9 & 98.0 & 85.0 & 0.1 \\
    \cline{1-7}
    \textbf{1PerFB}  & \textbf{\textsc{S2S+KD}}  & 94.6 & 99.8 & 96.0 &  94.0 & 0.1\\
    \cline{1-7}
    \textbf{1PerFBQ}  & \textbf{\textsc{S2S+KD+DDA}} & 95.8 & 100.0 & 99.3 & 85.0 & 0.1 \\
    \cline{1-7}
    \textbf{1PerFB}  & \textbf{\textsc{S2S+KD+DDA}}& 94.6 & 100.0 & 98.6 & 94.0 & 0.1 \\
    \cline{1-7}
    \end{tabularx}
  \vspace{-0.2cm}
   \caption{Results on all Time domain experiments. All metrics are percentages. }
     \label{tab:timeresultsall}%
     \vspace{-0.5cm}
\end{table*}%

 \vspace{1.5cm}

\begin{table*}[bh!]
  \small
  \begin{center}
    \begin{tabularx}{0.99\linewidth}{c|c|ccccc}
    \cline{1-7}
     \multirow{2}{*}{\textbf{Data}}& \multirow{2}{*}{\textbf{Approach}} & \textbf{BLEU} & \textbf{\textsc{Tree}} & \multirow{2}{*}{\textbf{Acceptability}} & \textbf{\textsc{Data}}& \textbf{\textsc{TreeAcc}}\\ 
     &  & \textbf{\textsc{Score}} & \textbf{\textsc{Accuracy}} &  & \textbf{\textsc{Reduction}}& \textbf{\textsc{STDev}}\\
    \cline{1-7}
    \textbf{ALL} &  \textbf{\textsc{S2S BASE}} & 92.6 & 99.3 & - & 0.0 & 0.1 \\
     \cline{1-7}
     \textbf{1PerCB} &  \textbf{\textsc{S2S}} & 15.9 & 0.1 & 0.6 & 99.3 & 0.2 \\
     \cline{1-7}
    \textbf{1PerMB} & \textbf{\textsc{S2S}} & 89.94 & 75.7 & 28.0 & 94.2 & 22.4 \\
     \cline{1-7}
    \textbf{5PerMB+Alarm}  & \textbf{\textsc{S2S+JT}} & 92.4 & 97.6 & 88.7 & 82.6 & 1.3 \\
     \cline{1-7}
     \textbf{3PerFB+Alarm} & \textbf{\textsc{S2S+JT}} & 92.6 & 98.1 & 86.0 & 82.0 & 2.2 \\
     \cline{1-7}
     \textbf{1PerFBQ+Alarm}  & \textbf{\textsc{S2S+JT}} & 92.8 & 97.6 & 88.0 & 80.0 & 0.9 \\
     \cline{1-7}
     \textbf{1PerFBQ}   & \textbf{\textsc{S2S}} & 92.1 & 95.6 & 83.3 & 80.0 & 0.3 \\
     \cline{1-7}
     \textbf{1PerFB} & \textbf{\textsc{S2S}} & 90.4 & 85.7 & 47.3 & 92.5 & 27.0 \\
     \cline{1-7}
    \textbf{1PerFBQ}  & \textbf{\textsc{S2S+DDA}} & 92.3 & 96.9 & 82.0 & 80.0 & 0.2 \\
     \cline{1-7}
    \textbf{1PerFB} & \textbf{\textsc{S2S+DDA}} & 92.1 & 96.3 & 84.0 & 92.5 & 26.0 \\
     \cline{1-7} 
     \textbf{1PerFBQ} & \textbf{\textsc{BART+DDA}} & 92.1 & 98.3 & 93.3 & 80.0 & 0.2 \\
     \cline{1-7}
      \textbf{1PerFB}  & \textbf{\textsc{BART+DDA}} & 91.5 & 97.1 & 86.7 & 92.5 & 1.6 \\
    \cline{1-7}
    \textbf{1PerFBQ} & \textbf{\textsc{S2S+KD}} & 92.6 & 98.7 & 92.0 & 80.0 & 0.2  \\
    \cline{1-7}
    \textbf{1PerFB}  & \textbf{\textsc{S2S+KD}} & 91.9 & 98.1 & 83.3 & 92.5 & 0.2  \\
    \cline{1-7}
    \textbf{1PerFBQ}  & \textbf{\textsc{S2S+KD+DDA}} & 92.6 & 98.9 & 96.0 & 80.0 & 0.2  \\
    \cline{1-7}
    \textbf{1PerFB}  & \textbf{\textsc{S2S+KD+DDA}} & 91.9 & 98.3 & 94.0 & 92.5 & 0.2  \\
    \cline{1-7}
    \end{tabularx}
  \end{center}
  \vspace{-0.2cm}
   \caption{Results on all Reminder domain experiments. All metrics are percentages. }
     \label{tab:reminderresultsall}%
     \vspace{-0.5cm}
\end{table*}%

 \vspace{1.5cm}

\begin{table*}[bh!]
  \small
  \centering
 %   \begin{tabularx}{0.99\linewidth}{c|c|ccccc}
    \begin{tabularx}{0.7\linewidth}{ @{} c | c | c c c c @{} }
    \cline{1-6}
     \multirow{2}{*}{\textbf{Data}}& \multirow{2}{*}{\textbf{Approach}} & \textbf{BLEU} & \textbf{\textsc{Tree}}  & \textbf{\textsc{Data}}& \textbf{\textsc{TreeAcc}}\\ 
      &  & \textbf{\textsc{Score}} & \textbf{\textsc{Accuracy}} & \textbf{\textsc{Reduction}}& \textbf{\textsc{STDev}}\\
     \cline{1-6}
     \textbf{ALL}   & \textbf{\textsc{S2S BASE}} & 91.4 & 91.4 & 0.0 & 0.1 \\
     \cline{1-6}
     \textbf{1PerCB}   & \textbf{\textsc{S2S}} & 88.1 & 77.9  & 91.2 & 2.6 \\
     \cline{1-6}
     \textbf{1PerMB}  &\textbf{\textsc{S2S}} & 90.7 & 90.6  & 74.8 & 0.3 \\
     \cline{1-6}
     \textbf{1PerFB}   & \textbf{\textsc{S2S}} & 91.3 & 91.4  & 40.0& 0.1 \\
     \cline{1-6}
    \textbf{1PerFB} & \textbf{\textsc{S2S+DDA}} & 91.3 & 91.1  & 40.0& 0.1 \\
     \cline{1-6}
    \textbf{0.5PerFB} & \textbf{\textsc{S2S+DDA}} & 89.8 & 86.6  & 85.0& 18.5 \\
     \cline{1-6}
    \textbf{0.25PerFB} & \textbf{\textsc{S2S+DDA}} & 87.3 & 77.8  & 92.5& 12.3 \\
     \cline{1-6} 
     \textbf{0.5PerFB} & \textbf{\textsc{BART+DDA}} & 90.2 & 89.9  & 85.0 & 1.7\\
     \cline{1-6}
      \textbf{0.25PerFB} & \textbf{\textsc{BART+DDA}}  & 89.2 & 86.2  & 92.5 & 1.8\\
    \cline{1-6}
    \textbf{0.5PerFB} & \textbf{\textsc{S2S+KD}} & 90.8 & 90.9 &  85.0 & 0.1\\
     \cline{1-6}
      \textbf{0.25PerFB} & \textbf{\textsc{S2S+KD}}  & 89.7 & 89.4  & 92.5 & 0.1\\
    \cline{1-6}
    \textbf{0.5PerFB} & \textbf{\textsc{S2S+KD+DDA}} & 90.8 & 91.0  & 85.0 & 0.1\\
     \cline{1-6}
      \textbf{0.25PerFB} & \textbf{\textsc{S2S+KD+DDA}}  & 89.8 & 89.8  & 92.5& 0.1\\
    \cline{1-6}
    \end{tabularx}
  \vspace{-0.2cm}
   \caption{Results on all Weather domain experiments. All metrics are percentages. }
     \label{tab:weatherresultsall}%
     \vspace{-0.5cm}
\end{table*}%

\bibliographystyle{coling}
\bibliography{coling2020}

\end{document}
